# Supplementary material for: High-fidelity adiabatic quantum computation using the intrinsic Hamiltonian of a spin system: Application to the experimental factorization of 291311
Source: arXiv:1706.08061 source file (2017-06-25)
Supplement: Supplementary file 1 [file Supplemental_Material.pdf]

# Supplemental Material

## THE ROBUSTNESS TO AMPLITUDE FLUCTUATIONS OF THE PULSES

In the main text, the adiabatic passage starts with the initial Hamiltonian

$$H_0 = \sigma_x^1 + \sigma_x^2 + \sigma_x^3, \tag{1}$$

and ends with the problem Hamiltonian modulated by ELM methods:

$$H_p = \frac{1}{2}\left(1.2\sigma_z^1\sigma_z^2 - 4.9\sigma_z^2\sigma_z^3 + 4\sigma_z^1\sigma_z^3\right). \tag{2}$$

The instantaneous Hamiltonian during the adiabatic passage is given by:

$$H(s) = (1-s)\underbrace{\left(\sigma_x^1 + \sigma_x^2 + \sigma_x^3\right)}_{H_0} + sH_p. \tag{3}$$

The adiabatic evolution of the system is approximated by $L$ discrete steps with $\tau$ the duration of each step. After the $l^{\text{th}}$ step, the state in the quantum register is

$$|\phi_l\rangle = U_l U_{l-1} \cdots U_1 |\phi_0\rangle, \tag{4}$$

where $U_l = e^{-iH(s_l)\tau}$ and $|\phi_0\rangle$ is the ground state of $H_0$. Here we choose $\tau = 0.05$ and use a linear interpolation with $s_l = 0.01 \times l, (l = 1, 2, ...100)$. The fidelity between $|\phi_l\rangle$ and the ground eigenstate of the instantaneous Hamiltonian $H(s_l)$ is shown in Fig. S1 (black line).

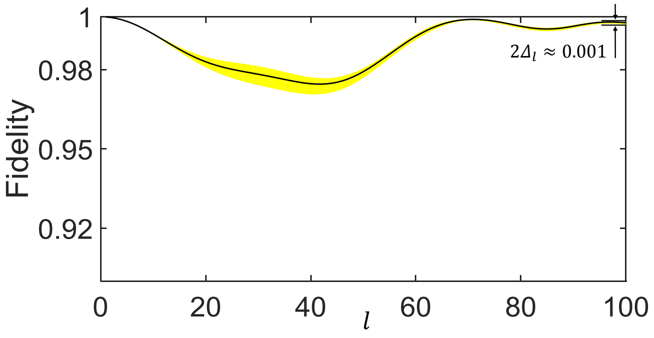


FIG. S1. The theoretical fidelities with the ground state of the instantaneous Hamiltonian during the adiabatic passage (black line). The yellow region labels the standard deviation of fidelities ($2\Delta_l$) when all the pulses have random amplitude fluctuations. The yellow band is asymmetric around the black curve because $F_l$ is slightly different from the black curve.

In our approach, the first term of $H(s_l)$ is simulated by radio-frequency pulses with amplitudes $\nu_l$. However, in the experiment the amplitudes inevitably have small fluctuations which lead to the effective Hamiltonian:

$$H^{\text{eff}}(s_l) = (1-s_l)((1+\delta_1)\sigma_x^1 + (1+\delta_2)\sigma_x^2 + (1+\delta_3)\sigma_x^3) + s_l H_p. \tag{5}$$

Here $\delta_1, \delta_2, \delta_3$ are independent random variables which have Gaussian distributions with expected values of 0 and standard deviations of 0.05. In this condition, the fidelity of the adiabatic passage will also have random fluctuations. For each $l$, we numerically analyzed the mean value of fidelities $F_l$ and the standard deviation $\Delta_l$. The yellow band in Fig. S1 represents the region $[F_l - \Delta_l, F_l + \Delta_l]$ for different $l$. The results show that although the pulses used in the experiments have fluctuations of around 5%, the standard deviation of the fidelity of the final state is smaller than 0.001.

## A COMPARISON WITH THE AVERAGE HAMILTONIAN METHOD

In this section we will compare the robustness of our method to the average Hamiltonian method.

Without energy landscape manipulation techniques, the problem Hamiltonian would be:

$$H_c = \frac{1}{2}\left(\sigma_z^1\sigma_z^2 - \sigma_z^2\sigma_z^3 + \sigma_z^1\sigma_z^3\right). \tag{6}$$

Here we choose the same initial Hamiltonian of the adiabatic evolution as

$$H_0 = \sigma_x^1 + \sigma_x^2 + \sigma_x^3. \tag{7}$$

The instantaneous Hamiltonian $H'(s)$ during the adiabatic passage is given by:

$$H'(s) = (1-s)\underbrace{\left(\sigma_x^1 + \sigma_x^2 + \sigma_x^3\right)}_{H_0} + s \cdot \underbrace{\frac{1}{2}\left(\sigma_z^1\sigma_z^2 - \sigma_z^2\sigma_z^3 + \sigma_z^1\sigma_z^3\right)}_{H_c}. \tag{8}$$

According to the average Hamiltonian theory and Trotter approximation, the evolution of $H'(s)$ for a certain time $\tau$ can be simulated with the pulse sequence in Fig. S2. The nuclear magnetic resonance sample used here is the same as the one in the main text (Fig. 1).

Although the evolution of $H'(s)$ can be simulated with a high fidelity, the quantum system actually exits the ground state during the implementation of this quantum circuit, which means the evolution is not truly adiabatic, and in fact is less robust. Ideally, the final state after the adiabatic evolution would have a fidelity of over 0.998 with the ground state of $H_c$ (Fig. S3). However, if all the pulses used in the quantum circuit suffer from amplitude fluctuation, the fidelity of adiabatic passage will fall off rapidly. Here we adopt the same noise model as above and find the fidelity of the final state will vary within the range $[0.866, 0.896]$ with standard deviation $\Delta \approx 0.015$ (Fig. S3). As a comparison, the theoretical fidelity of the

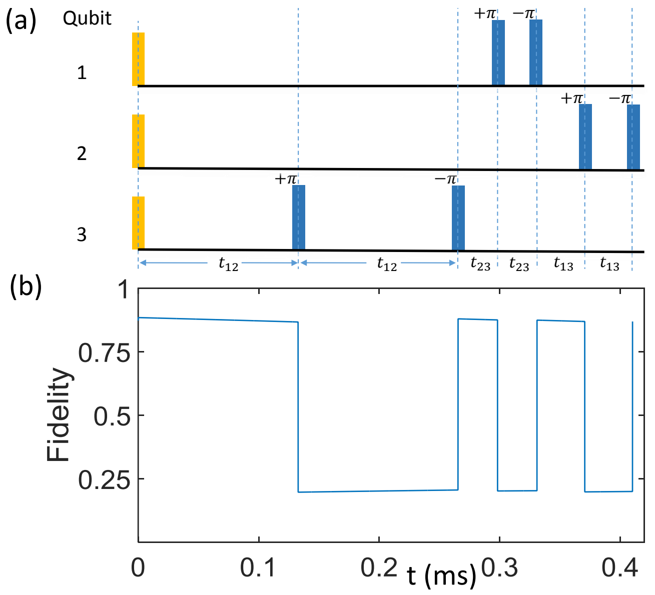


FIG. S2. (a)The pulse sequence for simulating the evolution of $H'(s)$ for a certain time $\tau$. Here the yellow blocks represent $e^{-i(1-s)\sigma_x\tau}$, and blue blocks labeled with $\pm\pi$ represent the decoupling pulses $e^{\pm i\pi\frac{\sigma_x}{2}}$. The evolution times are $t_{jk} = \frac{s\tau}{2\pi J_{jk}}$, and the coupling strengths $J_{jk}$ of the NMR sample are shown in Fig. 1 of the main text. (b) The theoretical fidelity with the ground state of $H'(s = 0.8)$, during the pulse sequence for simulating the evolution of $H'(s = 0.8)$.

final state by using the ELM method only varies within $[0.997, 0.998]$. Furthermore, in the average Hamiltonian method, the quantum system exits the ground state during certain segments (see Fig. S2, where the fidelity with the ground state falls below 0.25 during the pulse sequence for simulating the evolution of $H'(s = 0.8)$).

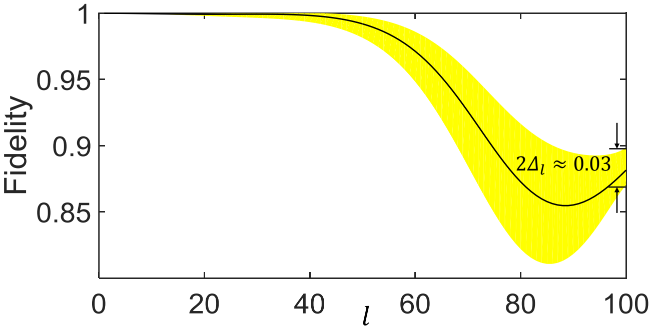


FIG. S3. The theoretical fidelities under ideal conditions with the ground state of the instantaneous Hamiltonian during the adiabatic passage (black line). The yellow region labels the standard deviation of fidelities ($2\Delta_l$) around the mean value $F_l$ for each $l$ when all the pulses have random amplitude fluctuations. The yellow band is asymmetric around the black curve because $F_l$ is slightly different from the black curve.

## THE EXPERIMENTALLY RECONSTRUCTED DENSITY MATRIX OF THE FINAL STATE

The real and imaginary parts of the reconstructed density matrix of the final state are shown in Fig. S4, with a fidelity of over 0.99 compared to the theoretical prediction. Here the fidelity between density matrix $\sigma$ and a quantum state $|\phi\rangle$ is defined as $F(\sigma, |\phi\rangle) = \langle\phi|\sigma|\phi\rangle/\sqrt{\mathrm{tr}(\sigma^2)}$.

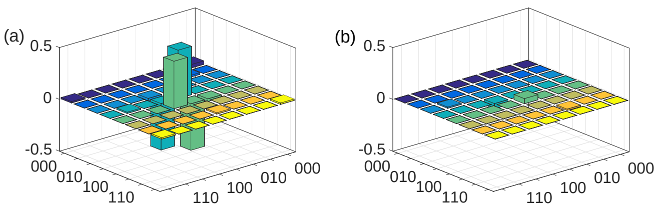


FIG. S4. The real (a) and imaginary (b) parts of the tomographically reconstructed density matrix of the final state after the adiabatic evolution. The experimental results have a fidelity of over 0.99 compared to the theoretical prediction, indicating a high accuracy of the quantum evolution in our experiments.

## CLASSICAL PRE-PROCESSING

Various papers have shown that prime factorization is equivalent to solving a set of simultaneous equations of binary variables [1–4]. Many variables in these equations can be eliminated by computationally cheap preprocessing steps. In this work the pre-processing has three steps: (1) apply simple judgments to each equation, (2) apply substitutions involving a small number of variables to each equation, and (3) apply small substitutions with a small number of variables to multiple equations at a time. Since each step simplifies the problem, we apply each step repeatedly until no more progress is made, before moving on to the next step.

*Step 1: Judgments.* We first expand the equations and re-arrange the terms so that we only have positive coefficients appearing. We then apply *judgments.* For the pre-processing of the equations that factorize 291311, the judgments that were involved are listed in Table S1. We note that Judgment 1 is a generalization of J1 appearing in the Supplemental Material of [3]. Judgments 2 and 3 in Table S1 are re-formulations of J2 and J3 from [3]. We further extended J1, J2, and J3 of [3] by allowing solutions of the form $z_1 = 1 - z_2$, which is equivalent to the negation of $z_2$, and in Table S1 we added newer judgments enumerated from 4 to 6, then we gave names for Judgments 1 to 6. We note that any asymmetric judgments are applied twice to the equations, swapping the left and right hand sides (LHS and RHS).

TABLE S1. List of Judgments

| Judgment | Description | Example |
| --- | --- | --- |
| 1. Double | If $z_1 + \ldots + z_n = 1$ then $z_i z_j = 0$ for all $1 \leq i < j \leq n$. | $z_1 + z_2 + z_3 = 1 \Rightarrow z_1 z_2 = z_2 z_3 = z_3 z_1 = 0$. |
| 2. MaxContradiction | Test to see if setting the term on the RHS with the largest positive coefficient to 1 would make max(LHS) < min(RHS). | $z_1 + z_2 = 2 + z_3 \Rightarrow z_3 = 0$. |
| 3. MinContradiction | Test to see if setting the term on the LHS to 0 would make max(LHS) < min(RHS). | $z_1 + 2z_2 = 2 + z_3 \Rightarrow z_2 = 1$. |
| 4. Product | If a product of variables is equal to 1, they must all be. | $z_1 z_2 z_3 = 1 \Rightarrow z_1 = z_2 = z_3 = 1$. |
| 5. MinMax | Compare the minimum value of one side with the maximum value of the other. If they are equal, we must have equality. | $z_1 + z_2 + z_3 = 3 \Rightarrow z_1 = z_2 = z_3 = 1$,<br>$z_1 + z_2 + z_3 = 0 \Rightarrow z_1 = z_2 = z_3 = 0$,<br>$z_1 + z_2 = 2 + z_3 \Rightarrow z_1 = z_2 = 1$ and $z_3 = 0$. |
| 6. Parity | Reduce the equation modulo 2. | $z_1 + 2z_2 + 4z_3 = 3 + 2z_4 \Rightarrow z_1 = 1$,<br>$z_1 + z_2 + 2z_3 = 3 \Rightarrow z_1 = 1 - z_2$. |

*Step 2: Substitutions involving a small number of variables in one equation.* One might notice that most of these *general* judgments can be derived by substituting values for certain variables into an equation and searching for contradictions. For a *specific* optimization problem (such as the one whose solution encodes the factors of 291311) we can do the same thing, and make significantly more progress in the pre-processing of the equations with further contradictions not covered by the general Judgments in Table S1. For a given equation, we can select a small number of variables and search for patterns within them, such as $z_3 = 0$, or $z_2 = 1 - z_5$, or $z_2 z_3 = 0$.

While Step 2 is very general and subsumes all of the previous judgments, it is more expensive if the number of variables considered gets large. However in this work, we only needed to apply this method to equations with fewer than 10 variables. We note that enumerating $2^{10}$ solutions amounts to only 1024 substitutions, and typical laptops can perform billions of operations per second. On laptop computers, experience tells us that we need to do substitutions involving more than 30 variables for it to take noticeable time, and the amount of pre-processing that can be accomplished by this stage can already be rather significant.

*Step 3: Substitutions involving a small number of variables in* ***many*** *equations.* The final step is the generalization of Step 2 to multiple equations. We enumerate all possible solutions for one equation, then substitute each of these solutions into a second equation. If there are any variables remaining we extend the solution by listing the possible values of the extra variables. We continue in this manner until the number of possible states exceeds a certain bound. Once the bound is reached, we search for patterns in our set of possible solutions, exactly as we did for Step 2. In theory, by setting the bound high enough, we would solve any problem by brute force since this is essentially a breadth first search of the solution space. However, in practice we choose to set the bound somewhere in between $2^{10}$ and $2^{50}$, depending on how much time we wish to allow for the pre-processing. In this particular example, $2^{20}$ was sufficient.

### Analysis for a number that has not yet been factored by a classical computer: RSA-230

We apply the three classical pre-processing steps discussed above to the factorization equations of RSA-230. This gives us a set of equations, involving at most quadratic terms. To express these as a minimization problem, we take the equations, each of the form $f_i = g_i$ for $1 \leq i \leq N$, and consider the Hamiltonian:

$$H = \sum_{i=1}^{N} \left(f_i - g_i\right)^2 . \tag{9}$$

Now $H$ is a quartic, which must be quadratized. While many techniques to do this exist, the least sophisticated method is to introduce new variables $z_{ij} = p_i q_j$ for $1 \leq i, j \leq n$, where $n$ is the bit-length of the factors, and substitute them into the original equations to form the linear equations: $\tilde{f}_i = \tilde{g}_i$. In general, this will introduce

roughly $n^2$ qubits (in fact it is slightly less as we will have solved some of the $p_i$ and $q_i$ during the pre-processing).

Now the factors of RSA-230 can be read from the global minima of the quadratic Hamiltonian:

$$\tilde{H} = \sum_{i=1}^{N} \left( \tilde{f}_i - \tilde{g}_i \right)^2 + \sum_{1 \leq i,j \leq n} \left( 3z_{ij} - 2p_i z_{ij} - 2q_j z_{ij} + p_i q_j \right) . \tag{10}$$

The last terms are added to ensure that $z_{ij} = p_i q_j$ at the global minima.

To get a very rough idea of an upper bound on the number of qubits needed for RSA-230, we have applied merely *Step 1*, followed by this simple (but not optimal) quadratization procedure, which gives us 5893 logical qubits and 148 776 qubits after quadratization. The entire pre-processing procedure took less than 200 minutes on a laptop. Considering that it took three years to factor RSA-220 [5], we believe that this pre-processing time is *vastly* less than the expected time it would take to factor RSA-230 (whether on a classical computer or a near-future quantum computer).


[1] C. J. Burges, Microsoft Research, Technical Report No.MSR-TR-2002-83 , **19** (2002).

[2] G. Schaller and R. Schutzhold, Quantum Inf. Comput. **10**, 0109 (2010).

[3] N. Xu, J. Zhu, D. Lu, X. Zhou, X. Peng, and J. Du, Phys. Rev. Lett. **108**, 130501 (2012).

[4] N. S. Dattani and N. Bryans, arXiv preprint arXiv:1411.6758 (2014).

[5] S. Bai, P. Gaudry, A. Kruppa, E. Thom, and P. Zimmermann. Private Communication. (2016).
